# Supplementary material for: Gaussian copula correlation network analysis of mixed-type data using a semi-parametric pairwise likelihood with a multi-omics application
Source: arXiv:2506.08586 source file (2026-11-18)
Supplement: Supplementary file 1 [file supplementary.tex]

\documentclass{article}

\usepackage{amsmath}
\usepackage{xcolor}
\usepackage{bbold}
\usepackage{graphicx}
\usepackage{subcaption}
\usepackage{float}
\usepackage{algorithm}
\usepackage{algpseudocode}
\usepackage{mathtools}
\usepackage{ragged2e}
\usepackage{subcaption}
\usepackage{enumerate}
\usepackage{natbib}
\usepackage{xr}

\renewcommand{\Pr}{\mathbb{P}}

\externaldocument{main}

\graphicspath{{./}} % {./figs/}

\title{Supplementary material for ``Gaussian copula correlation network analysis with application to multi-omics data'' by Tomilina, Jaffrézic and Mazo}

%%%%%%%%%%%%%%%%%%%%%%%%%%%%%%%%%%%%%%%%%%%%%%%%%%%%%%%%%%%
\begin{document}

\maketitle

\tableofcontents

\section{Supplementary Figures}

\begin{figure}[H]
  \begin{subfigure}{\textwidth}
  \centering
  \includegraphics[width=0.5\linewidth]{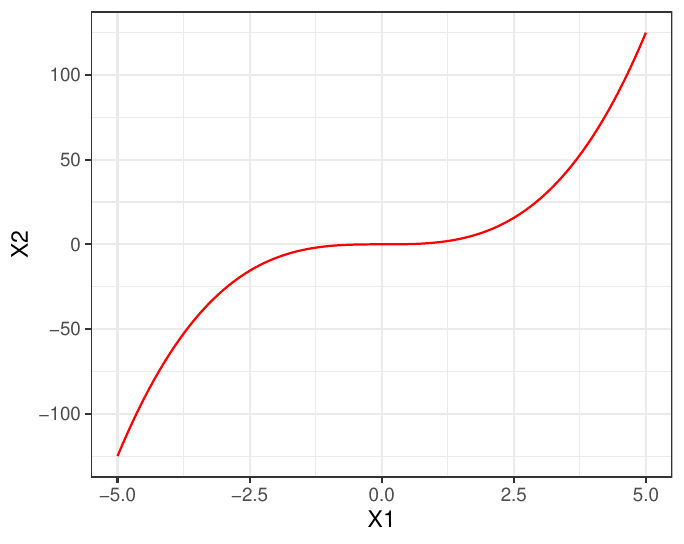}
  \caption{Case (i)}
\end{subfigure}
\begin{subfigure}{\textwidth}
  \centering
  \includegraphics[width=0.5\linewidth]{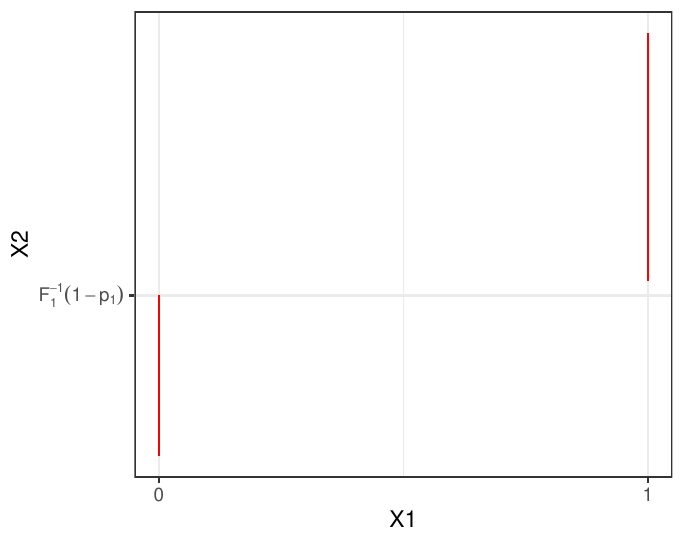}
  \caption{Case (ii)}
\end{subfigure}
  \begin{subfigure}{\textwidth}
  \centering
  \includegraphics[width=0.5\linewidth]{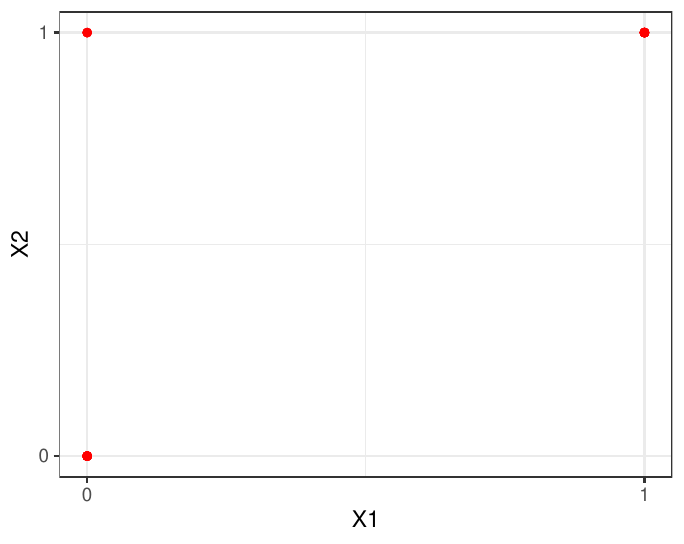}
  \caption{Case (iii)}
\end{subfigure}
  \caption{Illustration of comonotonicity for cases (i), (ii) and (iii) of Proposition \ref{prop:characterization}}
\label{fig:comonotonicity}
\end{figure}

\begin{figure}[H]
  \begin{subfigure}{\textwidth}
  \centering
  \includegraphics[width=0.5\linewidth]{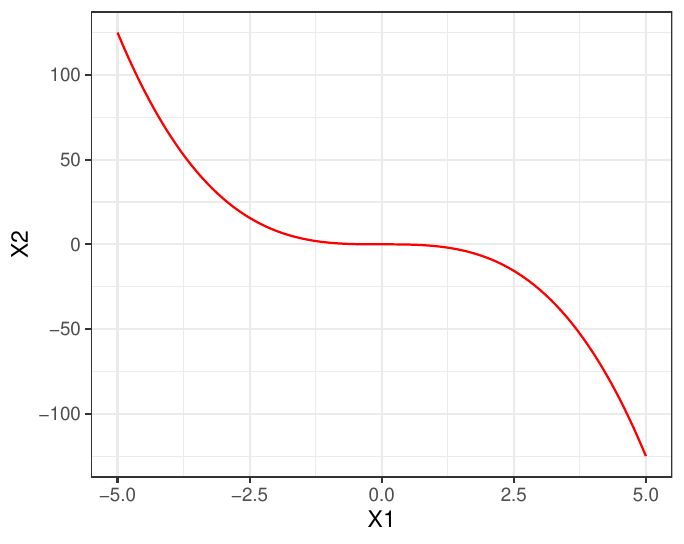}
  \caption{Case (i)}
\end{subfigure}
\begin{subfigure}{\textwidth}
  \centering
  \includegraphics[width=0.5\linewidth]{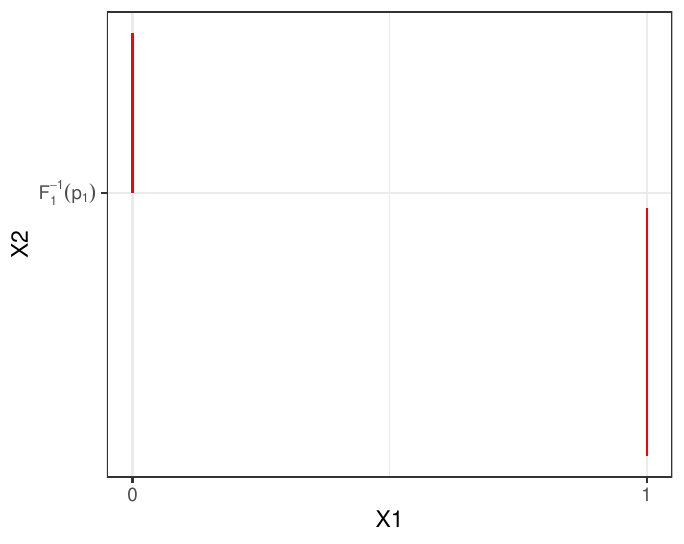}
  \caption{Case (ii)}
\end{subfigure}
  \begin{subfigure}{\textwidth}
  \centering
  \includegraphics[width=0.5\linewidth]{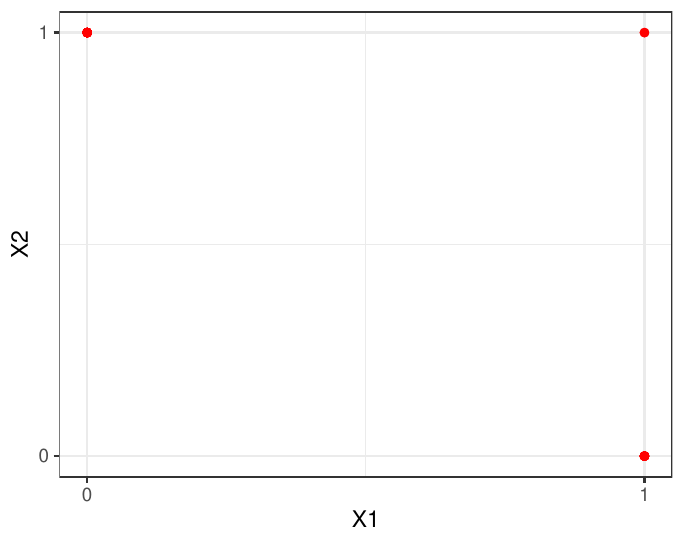}
  \caption{Case (iii)}
\end{subfigure} \caption{Illustration of countermonotonicity for cases (i), (ii) and (iii) of Proposition \ref{prop:characterization}}
\label{fig:countermonotonicity}
\end{figure}

\begin{figure}[H]
  \includegraphics[width=\linewidth]{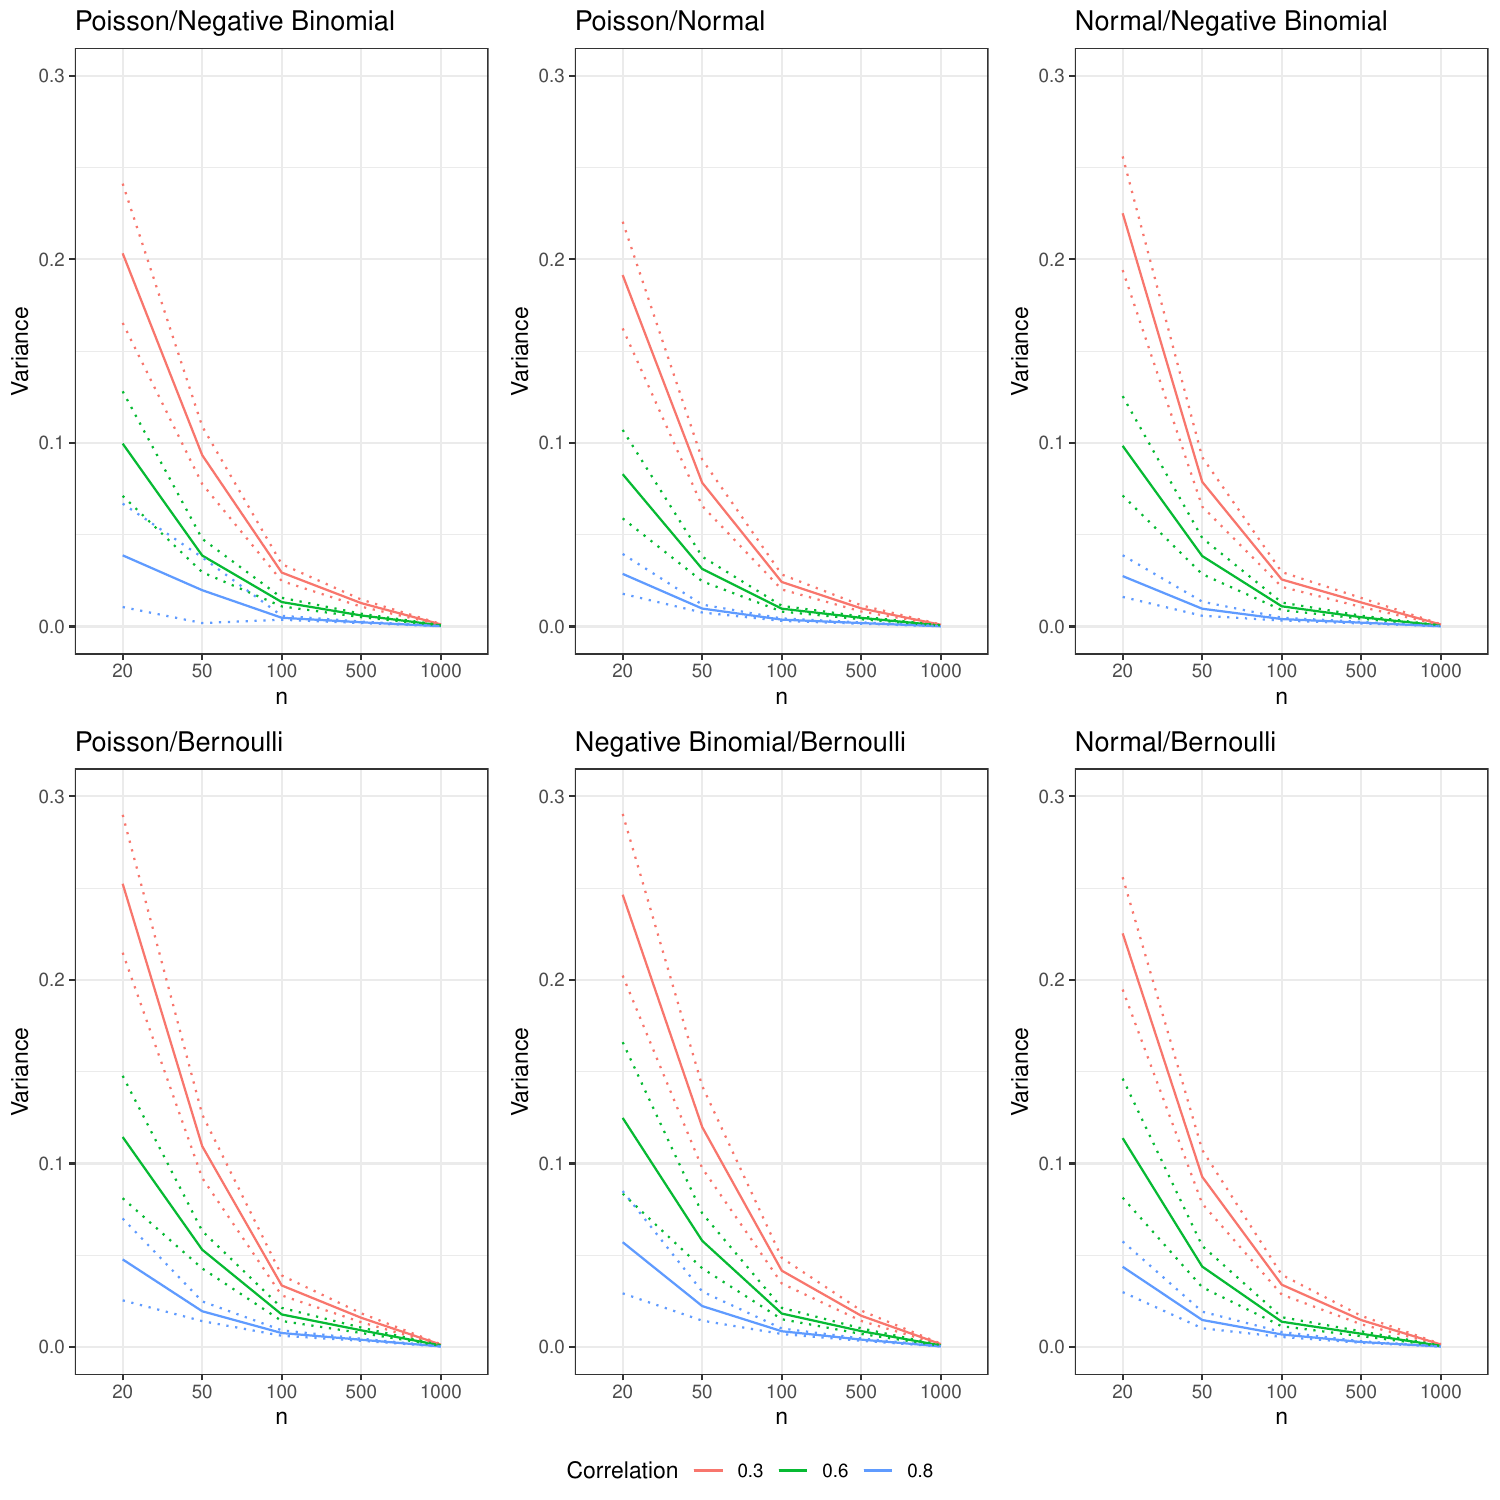}
  \caption{Averaged variances and 95\% confidence intervals (for N=500 replications) of the Gaussian copula correlation coefficient estimators defined in (\ref{eqn:estimator}) for $\rho = 0.3, 0.6, 0.8$ between $P(1)$, $NB(1,\frac{1}{2})$, $\mathcal{N}(0,1)$ and $\mathcal{B}(\frac{1}{2})$ depending on the sample size.}
\label{fig:pairwise_var}
\end{figure}

\begin{figure}[H]
  \includegraphics[width=\linewidth]{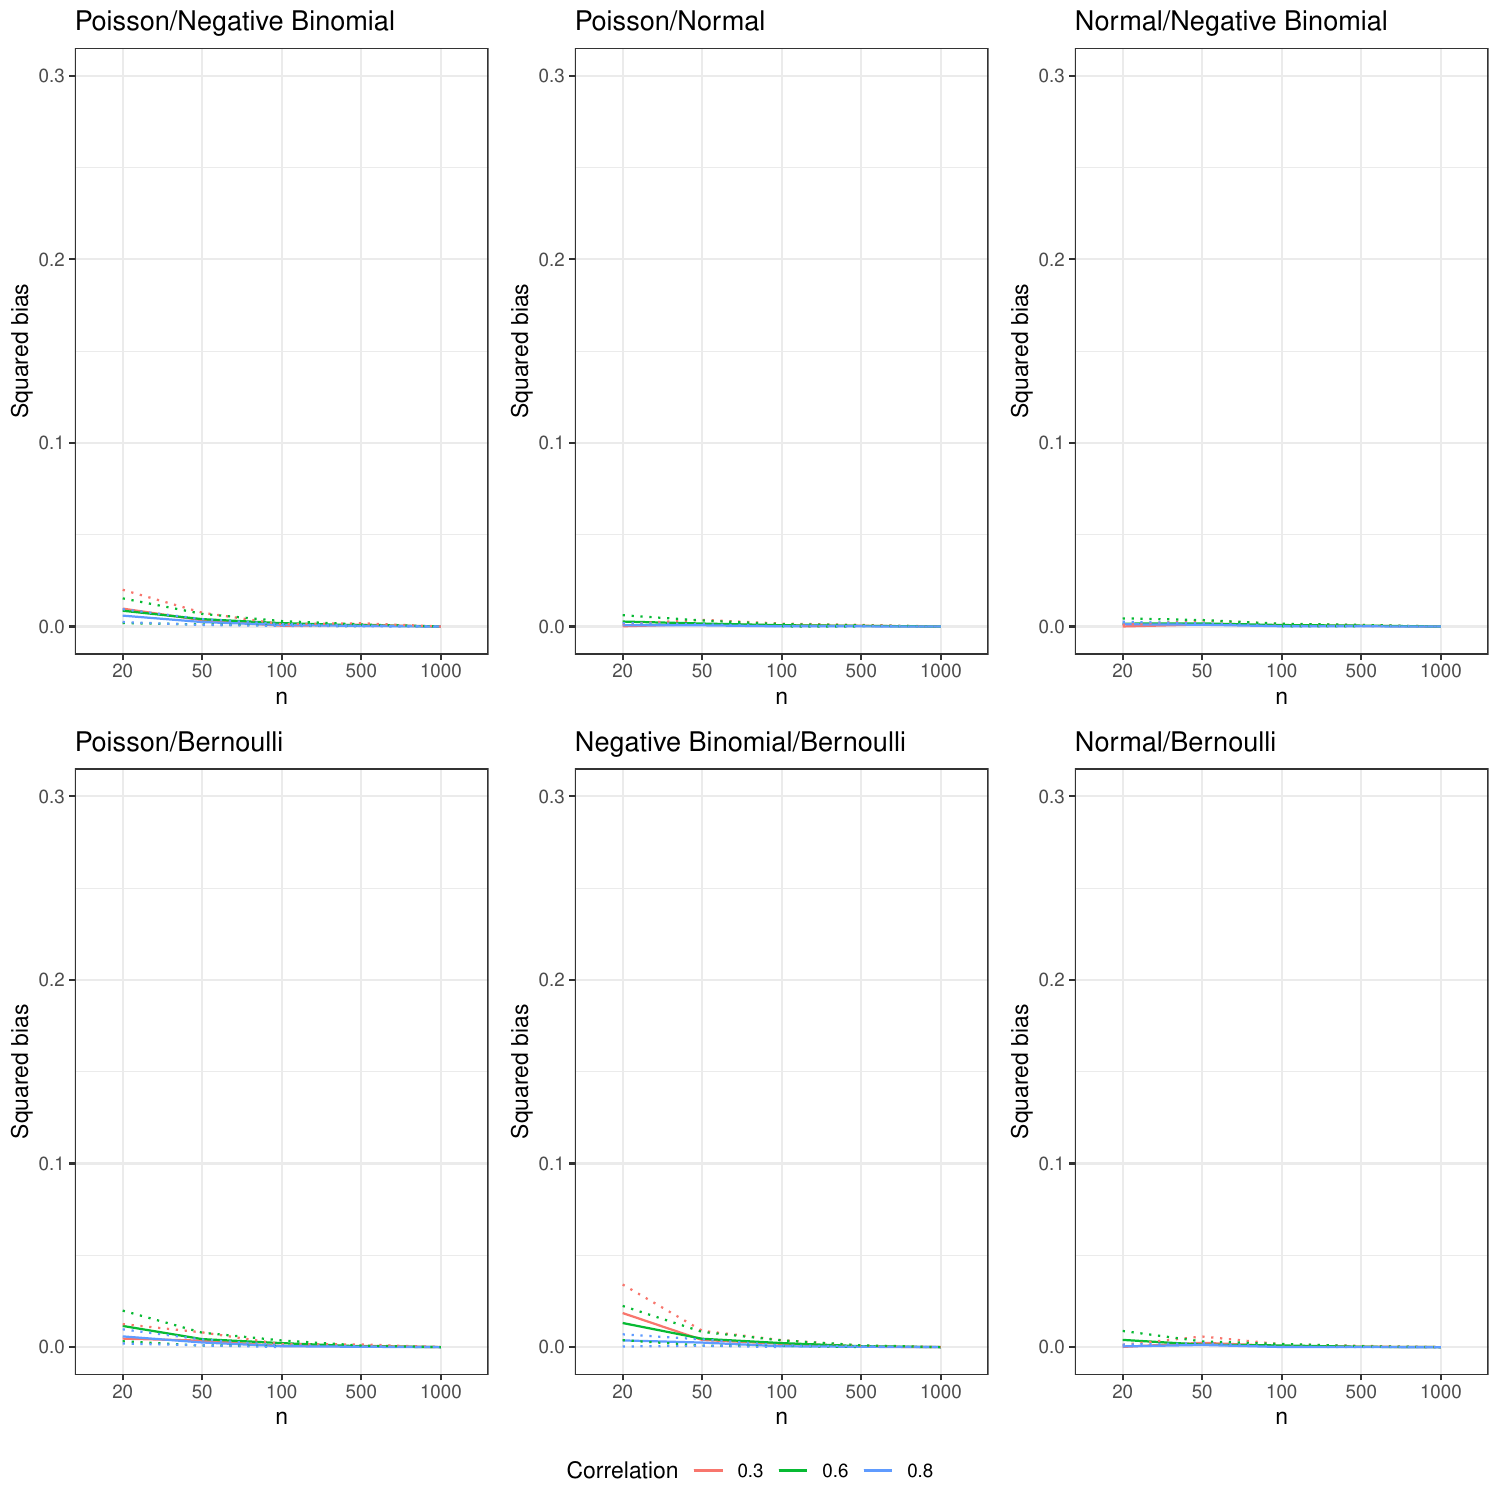}
  \caption{Averaged squared biases and 95\% confidence intervals (for N=500 replications) of the Gaussian copula correlation coefficient estimators defined in (\ref{eqn:estimator}) for $\rho = 0.3, 0.6, 0.8$ between $P(1)$, $NB(1,\frac{1}{2})$, $\mathcal{N}(0,1)$ and $\mathcal{B}(\frac{1}{2})$ depending on the sample size.}
\label{fig:pairwise_sqbias}
\end{figure}

\begin{figure}[H]
  \includegraphics[width=\linewidth]{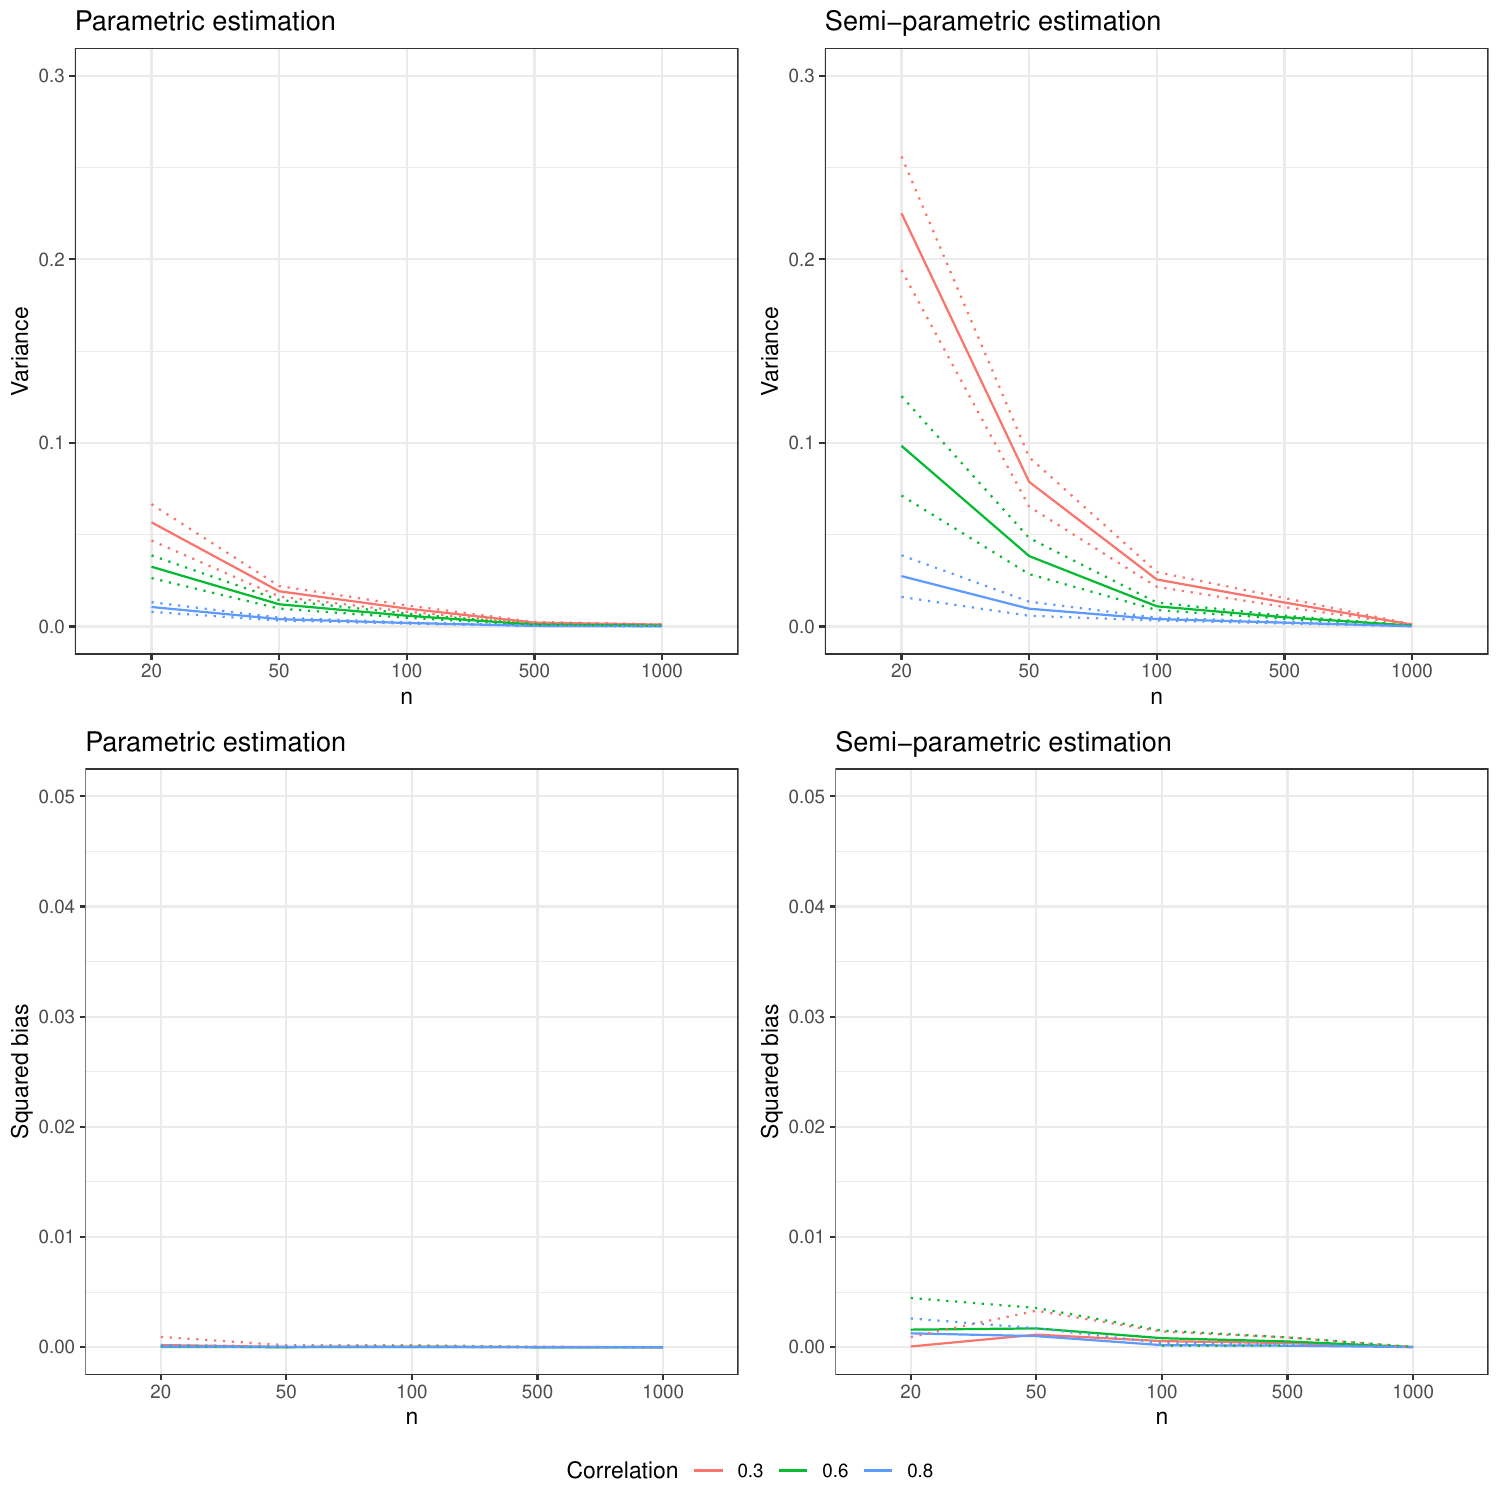}
  \caption{Averaged variances and squared biases with 95\% confidence intervals of $\hat\rho$ obtained with the semi-parametric method and the parametric method when the  marginals are correctly specified for different values of $\rho$ and sample sizes.}
  \label{fig:p_vs_np_right}
\end{figure}

\begin{figure}[H]
  \includegraphics[width=\linewidth]{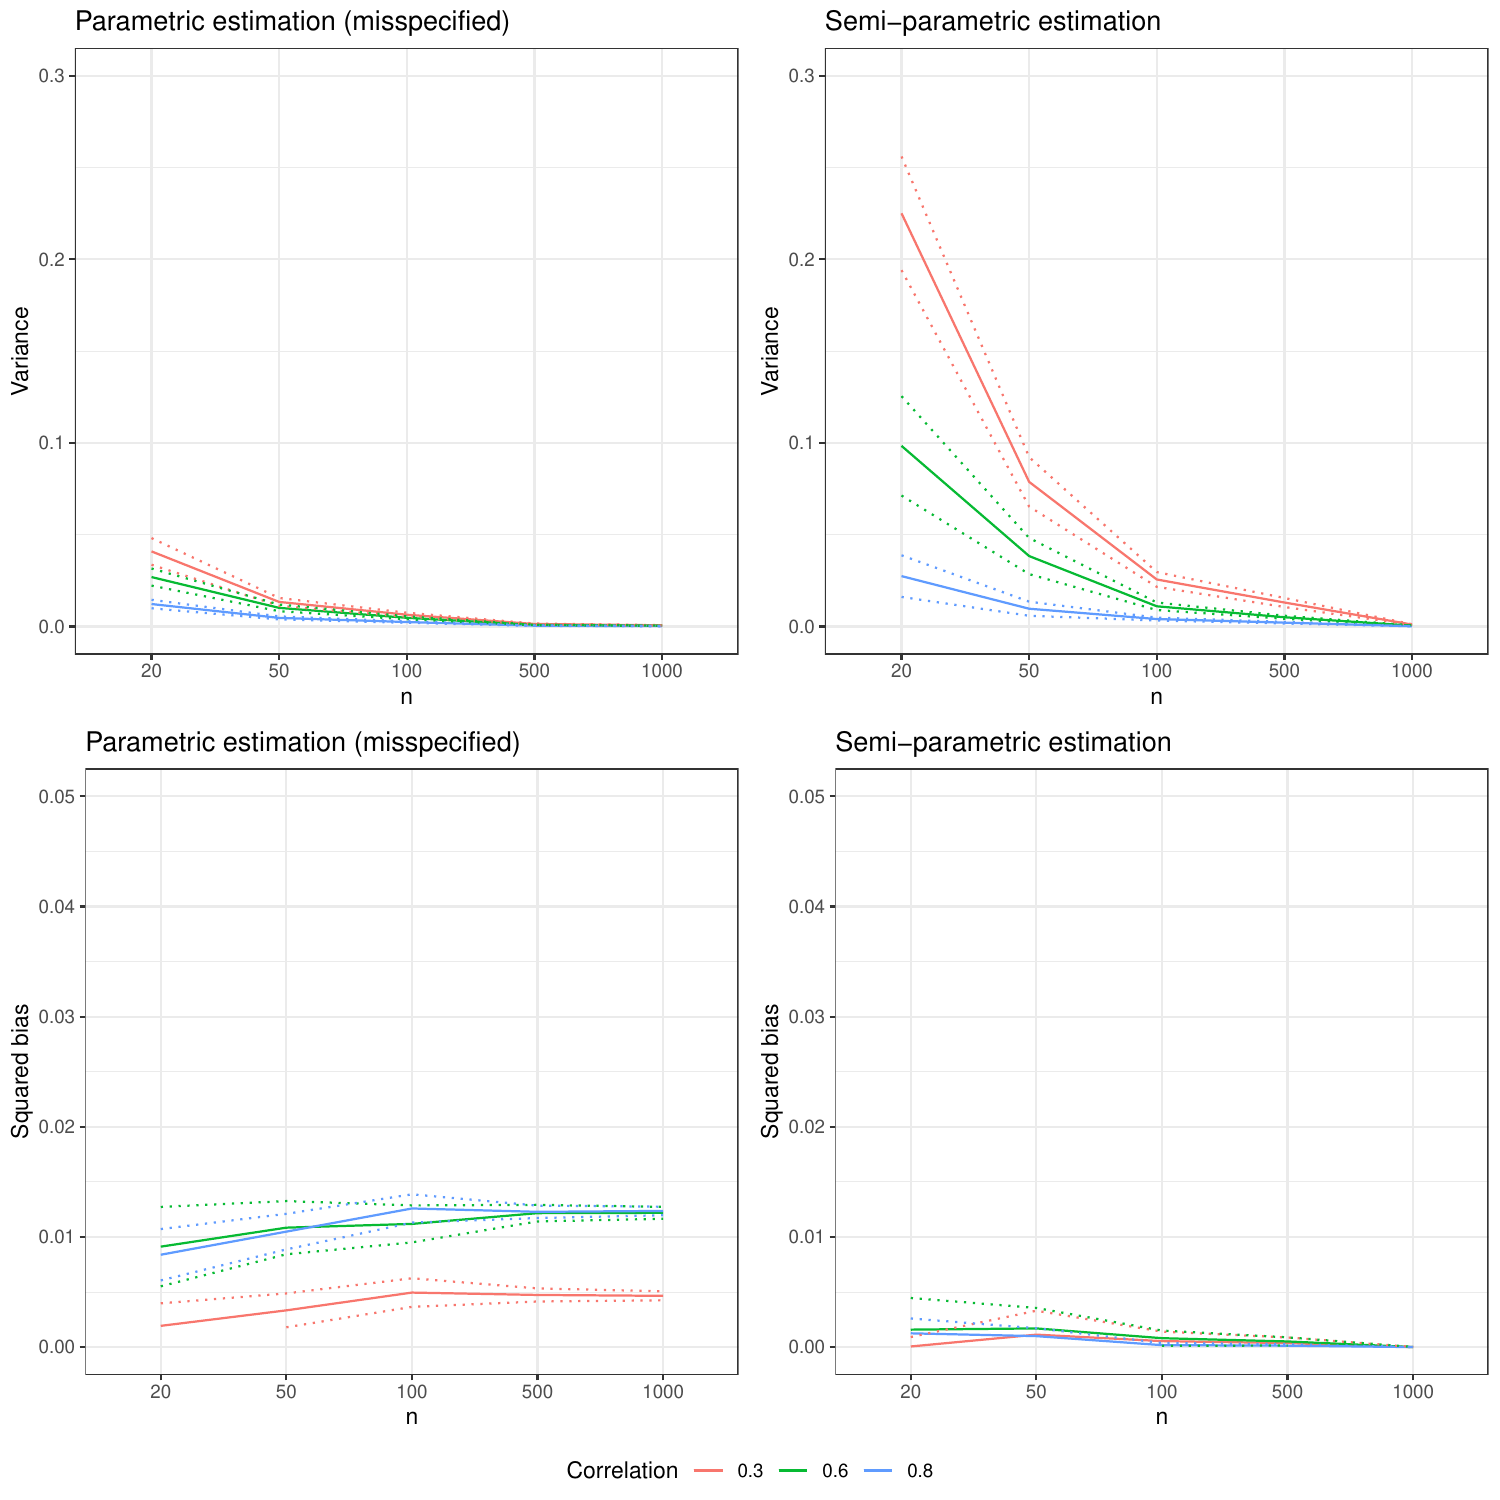}
  \caption{Averaged variances and squared biases with 95\% confidence intervals of $\hat\rho$ obtained with the semi-parametric method and parametric method when the marginals are misspecified for different values of $\rho$ and sample sizes.}
  \label{fig:p_vs_np_wrong}
\end{figure}

\begin{figure}[H]
  \centering
  \includegraphics[width=\linewidth]{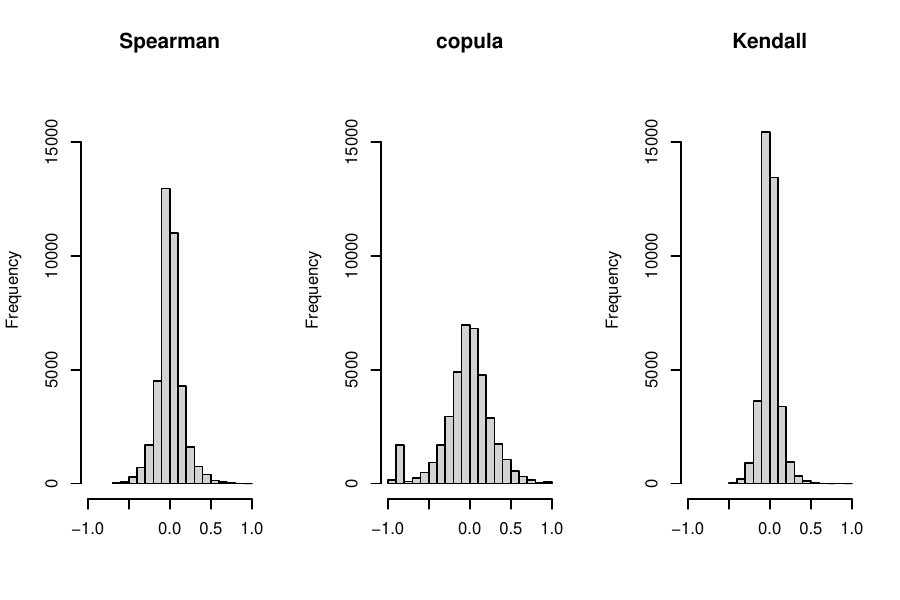}
\caption{Histograms of the estimated correlation coefficients for
  Spearman's $\rho^S$, the copula and Kendall's $\tau$.}
\label{fig:hist_coefs}
\end{figure}

\begin{figure}[H]
  \centering
  \includegraphics[width=0.99\linewidth,
  trim=2cm 0cm 2cm 0cm, clip=true]{network_s_AND_k.pdf}
    \caption{Kendall and Spearman
      networks for different threshold values. The nodes (variables)
      are colored by biological type (RNA-seq, protein, mutation). An
      edge is drawn between two nodes if the absolute value of the
      corresponding estimated correlation coefficient is above the
      threshold.}
  \label{fig:NetworksSpearmanKendall}
\end{figure}

\section{Supplementary Tables}

\begin{table}[H]
    \begin{subtable}[h]{\textwidth}
    \scalebox{0.85}{
    \begin{tabular}{|c|c|c|c|c|c|}
    \hline
    sample size & 20 & 50 & 100 & 500 & 1000\\
    \hline
    $\Sigma_{\text{blocks}}$ & 0.329 (0.02) & 0.188 (0.02) & 0.127 (0.01) & 0.054 (0.004) & 0.038 (0.003)\\
    \hline
    $\Sigma_{0.2}$ & 0.315 (0.02) & 0.187 (0.01)& 0.127 (0.01) & 0.054 (0.004) &0.038 (0.003)\\
    \hline
    $\Sigma_{0.5}$ & 0.332 (0.01) & 0.195 (0.01) & 0.132 (0.01) & 0.056 (0.004) &0.039 (0.002)\\
    \hline
    $\Sigma_{0.8}$ & 0.349 (0.02)& 0.2 (0.01)& 0.133 (0.01)& 0.057 (0.006)&0.04 (0.002)\\
    \hline
    \end{tabular}
    }
    \caption{Root Mean Squared Error (RMSE)}
    \label{table:RMSE}
    \end{subtable}
    
    \begin{subtable}[h]{\textwidth}
    \scalebox{0.85}{
    \begin{tabular}{|c|c|c|c|c|c|}
    \hline
    sample size & 20 & 50 & 100 & 500 & 1000\\
    \hline
    $\Sigma_{\text{blocks}}$ & 0.265 (0.02)  & 0.148 (0.01) & 0.102 (0.01) & 0.043 (0.005)& 0.03 (0.003)\\
    \hline
    $\Sigma_{0.2}$ & 0.262 (0.02) & 0.15 (0.01) & 0.101 (0.01)& 0.043 (0.003)&0.03 (0.007)\\
    \hline
    $\Sigma_{0.5}$ & 0.279 (0.02) &0.155 (0.01) &0.105 (0.007) &0.04 (0.003) &0.031 (0.002)\\
    \hline
    $\Sigma_{0.8}$ & 0.283 (0.01) & 0.16 (0.008)& 0.107 (0.005)& 0.045 (0.002)&0.032 (0.002)\\
    \hline
    \end{tabular}
    }
    \caption{Mean Average Error (MAE)}
    \label{table:MAE}
    \end{subtable}
    
    \caption{Average normalized Root Mean Squared Error (a) and normalized Mean Absolute Error (b) values for $N=500$ replications for the copula correlation pairwise estimator for $d=30$ variables, for a block-wise matrix and for three different matrices of respective sparsity $\gamma_F=0.2,0.5,0.8$, for different sample sizes. The simulation standard deviations are specified in parentheses.}
\end{table}

\begin{table}[H]
    \centering
    \scalebox{1}{
    \begin{tabular}{|c|c|c|c|c|}
    \hline
    sample size & 20 & 50 & 100 & 500 \\
    \hline
    RMSE & 0.354 (0.004) & 0.202 (0.002) & 0.136 (0.001) & 0.058 (0.0005)\\
    \hline
    MAE & 0.294 (0.003) & 0.162 (0.001) & 0.108 (0.0007) & 0.046 (0.0004) \\
    \hline
    \end{tabular}
    }
    \caption{Average normalized Root Mean Squared Error and normalized Mean Absolute Error values for $N=500$ replications for the copula correlation pairwise estimator for $d=300$ variables, for a matrix of sparsity $\gamma_F=0.8$, for different sample sizes. The simulation standard deviations are specified in parentheses.}
    \label{table:results300}
\end{table}

\begin{table}[H]
    \centering
    \scalebox{1}{
    \begin{tabular}{|l|c|c|}
    \hline
    & Predicted zero & Predicted non-zero \\
    \hline
    Real zero  &  True negatives (TN) & False positives (FP)\\
    \hline
    Real non-zero & False negatives (FN) & True positives (TP)\\
    \hline
    \end{tabular}
    }
    \caption{Contingency matrix}
    \label{table:contingency_matrix}
\end{table}

\begin{table}[H]
    \centering
    \scalebox{0.8}{
    \begin{tabular}{|c|c|c|c|c|c|c|}
    \hline
    p&sample size & 20 & 50 & 100 & 500 & 1000\\
    \hline
    30&$\Sigma_{\text{blocks}}$ & 0.91 (0.04) & 0.97 (0.01) & 0.99 (0.007)& 0.999 (0.0004)& 0.999 (0.0005)\\
    \hline
    30&$\Sigma_{0.2}$ & 0.72 (0.03) & 0.82 (0.02)& 0.89 (0.02) & 0.96 (0.01) &0.98 (0.004)\\
    \hline
    30&$\Sigma_{0.5}$ &  0.76 (0.04) &0.88 (0.03) &0.94 (0.01) &0.99 (0.003)&0.994 (0.002)\\
    \hline
    30&$\Sigma_{0.8}$ & 0.84 (0.03)& 0.94 (0.02)& 0.98(0.01)&0.999 (0.001) &0.999(0.0004)\\
    \hline
    300&$\Sigma_{0.8}$ & 0.79 (0.01) & 0.90 (0.007) & 0.97 (0.004) & 0.998 (0.0002) & NE\\
    \hline
    \end{tabular}}
    \caption{Average AUC values for $N=500$ simulations for the copula pairwise correlation coefficients for different sample sizes. Four different sparse matrices were evaluated for $d=30$ variables (block-wise matrix, final sparsity $\gamma_F=0.2, 0.5, 0.8$). A matrix of sparsity $\gamma_F=0.8$ was considered for $d=300$ variables. The standard deviations are specified in parentheses, and the NE acronym stands for Not Evaluated.}
    \label{fig:AUC}
\end{table}

\begin{table}[H]
\centering
\begin{subtable}[h]{0.3\textwidth}
\centering
\scalebox{1}{
\begin{tabular}{|c|c|c|}
    \hline
     &  0 & 1 \\
     \hline
     0 & 437156 & 5723\\
     \hline
     1& 7621 & 0\\
     \hline
\end{tabular}
}
\caption{}
\label{table:cont_coef1}
\end{subtable}
\begin{subtable}[h]{0.3\textwidth}
\centering
\scalebox{1}{
\begin{tabular}{|c|c|c|}
    \hline
    & 0 & 1 \\
    \hline
    0 &  248 & 0 \\
    \hline
    1& 0 & 2 \\
    \hline
\end{tabular}
}
\caption{}
\label{table:cont_coef2}
\end{subtable}
\begin{subtable}[h]{0.3\textwidth}
\centering
\scalebox{1}{
\begin{tabular}{|c|c|c|}
    \hline
    & 0 & 1 \\
    \hline
    0 &  213 & 0 \\
    \hline
    1& 35 & 2 \\
    \hline
\end{tabular}
}
\caption{}
\label{table:cont_coef3}
\end{subtable}
\caption{Contingency tables for the mutation variables corresponding to the points for which the copula correlation coefficient was close to -1 (\ref{table:cont_coef1}) (1802 points), for which both the copula and Spearman had correlation coefficients of 1 (\ref{table:cont_coef2}) (one point), and for which the copula had a correlation coefficient close to 1 and Spearman close to 0 (\ref{table:cont_coef3}) (one point).}
\label{table:contingency}
\end{table}

\begin{table}[H]
    \centering
    \scalebox{1}{
    \begin{tabular}{|c|c|}
    \hline
     Variable & Gene \\
    \hline
     MU4777833 & ARHGEF11 \\
    \hline
    MU5153080 & SLC7A9  \\
    \hline
    MU17289 & CDKN1B  \\
    \hline
    MU5551967 & PQBP1 \\
    \hline
    \end{tabular}
    }
    \caption{Mutation variables with a degree greater than 10 in the copula correlation network for a threshold value of 0.7, and their corresponding genes.}
    \label{table:gene_mut}
\end{table}

\section{Proofs of Propositions}
\subsection{Proof of Proposition \ref{prop:density}}
\label{appendix:density}
  We are going to show that $f(x_1, ..., x_d)$ from equation (\ref{eqn:density}) corresponds to the density of the joint cumulative distribution $F(x_1, \dots, x_d)$ from model (1) with respect to the $\lambda^{\otimes p}\otimes\mu^{\otimes (d-p)}$ measure, where $\lambda^{\otimes p}=\underbrace{\lambda\times\dots\times\lambda}_{p\text{ times}}$ with $\lambda$ the Lebesgue measure and $\mu^{\otimes (d-p)}=\underbrace{\mu\times\dots\times\mu}_{d-p\text{ times}}$ denotes the counting measure. For easier notations, we denote $S^{a,b}$ , where $a<b$ and $a,b \in \{1, \dots, d\}$, the set $]-\infty;x_a]\times...\times]-\infty;x_b]$. Let us find $f$ that satisfies:
\begin{eqnarray}
    C_\Sigma(F_1(x_1), ..., F_d(x_d))&=&\int_{S^{1,d}}f(y_1, ..., y_d)\mathrm{d}(\lambda^{\otimes p}\otimes\mu^{\otimes (d-p)})(y_1, ..., y_d)\nonumber \\
    &=&\int_{S^{1,p}}\left(\int_{S^{p+1,d}}f(y_1, ..., y_d)\mathrm{d}\mu^{\otimes (d-p)}(y_{p+1}, ..., y_d)\right)\mathrm{d}\lambda^{\otimes p}(y_1, ..., y_p). \nonumber
\end{eqnarray}
The second equality can be directly obtained by Fubini-Tonelli's theorem. By differentiating both sides with respect to the $p$ continuous variables, we get:
\begin{eqnarray}
    \prod_{k=1}^{p}f_k(x_k)C^p_\Sigma(F_1(x_1), ...,F_d(x_d))&=&\int_{S^{p+1,d}}f(x_1, ..., x_p, y_{p+1}..., y_d)\mathrm{d}\mu^{\otimes (d-p)}(y_{p+1}, ..., y_d)\nonumber\\
    &=& \sum_{\substack{y_{p+1} \leq x_{p+1} \\ y_{p+1}\in S_{p+1}}} \dots \sum_{\substack{y_d \leq x_d \\ y_d \in S_d}} f(x_1, ..., x_p, y_{p+1}, ... y_d) \nonumber
\end{eqnarray}
where $f_j$ denotes the density of $X_j$, $C_\Sigma^p$ denotes the differential of $C_\Sigma$ with respect to the $p$ continuous variables, and $S_j$ denotes the support of $F_j$.
The Möbius inversion formula~\citep{rota1964} provides us with the following expression
\begin{eqnarray}
    f(x_1, ..., x_d)&=&\sum_{\substack{y_{p+1} \leq x_{p+1} \\ y_{p+1}\in S_{p+1}}}\dots \sum_{\substack{y_d \leq x_d \\ y_d \in S_d}}\prod_{k=1}^{p}f_k(x_k)C^p_\Sigma(F_1(x_1), ..., F_p(x_p), F_{p+1}(y_{p+1}), ..., F_d(y_d)) \nonumber \\
    && \hspace{3 cm} \times m_{p+1}(y_{p+1},x_{p+1})\cdots m_d(y_d,x_d) \nonumber
\end{eqnarray}
where
$$m_j(y_j,x_j) = \left\{
    \begin{array}{ll}
    1  & \mbox{if } x_j=y_j\\
    -1 & \mbox{if } y_j \mbox{ precedes } x_j \mbox{ in } S_j\\
    0  & \mbox{ otherwise. }
    \end{array}
\right.$$
In our case, one can notice that $y_j$ can only take the values $x_j$ and $x_j-$, where $x_j-$ denotes the point that precedes $x_j$ in $S_j$.  It corresponds to the expression of the multivariate density below where 
$$u_{k,j_k} = \left\{
    \begin{array}{ll}
    F_k(x_k) & \mbox{if } j_k=0\\
    F_k(x_k-) & \mbox{if } j_k=1\\
    \end{array}
\right.$$

$$f(x_1, \dots ,x_d)=\prod_{k=1}^{p}f_k(x_k)\sum_{j_{p+1}=0}^1... \sum_{j_d=0}^1(-1)^{j_{p+1}+\dots + j_d} \times C^p_\Sigma(F_1(x_1), ..., F_p(x_p), u_{p+1,j_{p+1}}, ..., u_{d,j_d})$$
The density is unique up to all sets of measure zero with respect to our measure $\lambda^{\otimes p} \otimes \mu^{\otimes d-p}$.

\subsection{Proof of Proposition \ref{prop:block_wise}}
\label{appendix:block_wise}
Let us show first that if the correlation matrix of the copula is of
the form
$$\Sigma=
\begin{pmatrix}
\Sigma_1 & 0 & 0\\
0 & ... & 0\\
0 & 0 & \Sigma_k
\end{pmatrix}$$
then the multivariate density can be factorized as
\begin{equation}\label{eq:density-factorizes}
  f(x_1, \dots,
  x_d)=\prod_{i=1}^k g_i(x_{G_i})
\end{equation}
for some functions $g_i$,
$i=1,\dots,k$. 
We know that for all $(u_1, \dots, u_d) \in (0,1)^d$,
\begin{eqnarray}
\label{eqn:deriv}
    \dfrac{\partial^p C_\Sigma(u_1, \dots, u_d)}{\partial u_1 \dots \partial u_p}&=&\int_{0}^{u_{p+1}}\dots\int_{0}^{u_d} |\Sigma|^{-\frac{1}{2}}\exp\left(-\dfrac{1}{2}\mathbf{v}^T(\Sigma^{-1}-I)\mathbf{v}\right)\mathrm{d}q_{p+1}\dots \mathrm{d}q_d
\end{eqnarray}
where $\mathbf{v}=(v_1, \dots, v_d)$ such that
\begin{equation*}v_i=\begin{cases}
    \Phi^{-1}(u_i) \text{ if }i \in \{1, \dots, p\}\\
    \Phi^{-1}(q_i) \text{ if }i \in \{p+1, \dots, d\}
\end{cases}\end{equation*}
and $I$ denotes the identity matrix.
Let us split the vector $\mathbf{v}$ as $\mathbf{v}^T=(\mathbf{v}_1^T, \dots, \mathbf{v}_k^T)$ where each $\mathbf{v}_l$ is of size $|G_l|\times 1$. Hence, the right-hand side of (\ref{eqn:deriv}) can be written as \begin{eqnarray}
\label{eqn:facto}
    &&\int_{0}^{u_{p+1}}\dots\int_{0}^{u_d} \left( \prod_{l=1}^k|\Sigma_l|^{-\frac{1}{2}}\exp\left(-\dfrac{1}{2}\mathbf{v}_l^T(\Sigma_l^{-1}-I |_{G_l})\mathbf{v}_l\right)\right)\mathrm{d}q_{p+1}\dots \mathrm{d}q_d
\end{eqnarray} where $I |_{G_l}$ denotes the identity matrix of size $|G_l|$.
By noticing that the $l$th factor only depends on $\mathbf{v}_l$, and
that each $q_j$ can only belong to exactly one $\mathbf{v}_l$,
Fubini-Tonelli's theorem enables us to factor (\ref{eqn:deriv}). Let
us denote by $\mathcal{D}(G_l)$ the set of indexes corresponding to
the discrete variables in $G_l$, that is $\mathcal{D}(G_l)=\{p+1,
\dots, d\}\cap G_l$. Denote $d_l = |\mathcal{D}(G_l)|$. We get that (\ref{eqn:facto}) can be written as
\begin{equation*}
    \prod_{l=1}^k \int_{0}^{u_{j_1(l)}} \cdots \int_{0}^{u_{j_{d_l}(l)}} |\Sigma_l|^{-\frac{1}{2}}\exp\left(-\dfrac{1}{2}\mathbf{v}_l^T(\Sigma_l^{-1}-I |_{G_l})\mathbf{v}_l\right)\mathrm{d}q_{j_{d_l}(l)}\cdots\mathrm{d}q_{j_{1}(l)}, 
\end{equation*}
where above $j_1(l),\dots,j_{d_l}(l)$ is an enumeration of the
elements of $\mathcal{D}(G_l)$. We use the convention that an integral over the empty set $\mathcal{D}(G_l)=\emptyset$ is replaced by its integrand. 
Let us define
\begin{equation*}
  P_l(\mathbf{u}_{\mathcal{C}(G_l)},\mathbf{u}_{\mathcal{D}(G_l)})=
\int_{0}^{u_{j_1(l)}} \cdots \int_{0}^{u_{j_{d_l}(l)}}
|\Sigma_l|^{-\frac{1}{2}}\exp\left(-\dfrac{1}{2}\mathbf{v}_l^T(\Sigma_l^{-1}-I|_{G_l}))\mathbf{v}_l\right)
\mathrm{d}q_{j_{d_l}(l)}\cdots\mathrm{d}q_{j_{1}(l)},
\end{equation*}
where  $\mathcal{C}(G_l)$ is the set of indexes corresponding to the
continuous variables in group $G_l$,
$\mathbf{u}_{\mathcal{D}(G_l)}=\{u_j : j \in \mathcal{D}(G_l) \}$ and
$\mathbf{u}_{\mathcal{C}(G_l)}=\{u_j : j \in \mathcal{C}(G_l)
\}$. Thus, remembering the notation $C_{\Sigma}^p(u_1,\dots,u_d)
\equiv \partial^p C/\partial u_1\cdots\partial u_p$, we have got
\begin{equation}\label{eq:factorization}
C_{\Sigma}^p(u_1,\dots,u_d) =
\prod_{l=1}^kP_l(\mathbf{u}_{\mathcal{C}(G_l)},\mathbf{u}_{\mathcal{D}(G_l)})
\end{equation}
for all $(u_1,\dots,u_d) \in \mathbb{R}^d$.
Choose and fix $(x_1,\dots,x_d) \in \mathbb{R}^d$. Remember that we
want to prove~(\ref{eq:density-factorizes}) for some functions $g_i$.
From~\eqref{eqn:density} in the main text, we have
\begin{multline*}
  f(x_1, \dots, x_d)=\\\left(\prod_{k=1}^{p}f_k(x_k)\right)
  \left(    \sum_{\alpha_{p+1}=0}^{1}\cdots\sum_{\alpha_d=0}^{1}
    (-1)^{\alpha_{p+1}+\cdots+\alpha_d}
     C_{\Sigma}^{p}(\zeta(1,0), \dots,
    \zeta(p,0),\zeta(p+1,\alpha_{p+1}),\dots,\zeta(d,\alpha_d)) \right),
  \end{multline*}
where each $\zeta$ is seen as a function on $\{p+1,\dots,d\} \times
\{0,1\}$ such that
$\zeta(i,0) = F_i(x_i)$ and $\zeta(i,1) =
F_i(x_i-)$. By~(\ref{eq:factorization}), we have
\begin{multline*}
  C_{\Sigma}^{p}(\zeta(1,0), \dots,
  \zeta(p,0),\zeta(p+1,\alpha_{p+1}),\dots,\zeta(d,\alpha_d))\\=
  \prod_{l=1}^k P_l(\zeta(i_1(l),0),\dots,\zeta(i_{c_l}(l),0),
  \zeta(j_1(l),\alpha_{j_1(l)}),\dots,
  \zeta(j_{d_l}(l),\alpha_{j_{d_l}(l)}))
  =: \prod_{l=1}^k P_l(\boldsymbol{\alpha}_{\mathcal{D}(G_l)}),
\end{multline*}
where above $i_1(l),\dots,i_{c_l}(l)$ is an enumeration of the
elements of $\mathcal{C}(G_l)$ with $c_l=|\mathcal{C}(G_l)|$.
It follows
\begin{eqnarray*}
    f(x_1, \dots, x_d)&=&\prod_{i=1}^p f_i(x_i) \sum_{\alpha_{p+1}=0}^1 \dots \sum_{\alpha_d=0}^1 (-1)^{\alpha_{p+1}+\dots+\alpha_d}\prod_{l=1}^k P_l(\boldsymbol{\alpha}_{\mathcal{D}(G_l)})\\
    &=&\left(\prod_{l=1}^k \prod_{i \in
        \mathcal{C}(G_l)}f_i(x_i)\right)\sum_{\alpha_{p+1}=0}^1
        (-1)^{\alpha_{p+1}}\dots \sum_{\alpha_d=0}^1 (-1)^{\alpha_d}\prod_{l=1}^k P_l(\boldsymbol{\alpha}_{\mathcal{D}(G_l)}) \\
&=&\prod_{l=1}^k \left( \prod_{i \in \mathcal{C}(G_l)}f_i(x_i)
    \sum_{\substack{\alpha_m=0 \\ m \in \mathcal{D}(G_l)}}^1
  (-1)^{\sum_{\alpha_m \in \mathcal{D}(G_l)}\alpha_m}P_l(\boldsymbol{\alpha}_{\mathcal{D}(G_l)})\right).
\end{eqnarray*}
This proves that the multivariate density $f$ factorizes.

Conversely, this factorization implies a k-block-diagonal structure
for $\Sigma$ by unicity of the density with respect to the product
measure $\underbrace{\lambda\times\dots\times\lambda}_{p\text{
    times}}\times\underbrace{\mu\times\dots\times\mu}_{d-p\text{
    times}}$.
The proof of Proposition~\ref{prop:block_wise} is complete.

\subsection{Proof of Proposition \ref{prop:characterization}}
\label{appendix:characterization}

Case~(i) is well-known and hence not shown here. Let us show 
cases~(ii) and~(iii). Remember that for all $0\le s \le 1$ and
$t\in\mathbb{R}$, it holds $F_j(F_j^\leftarrow(s)) \ge s$,
$F_j^\leftarrow(s) \le t$ if and only if $s\le F_j(t)$,
and $F_j(t)<s$ if and only if
$t<F_j^{\leftarrow}(s)$; see e.g.,~\citet{resnick}. Observe also that if
$X_j\sim\mathcal{B}(p_j)$ then
\begin{equation*}
  F_j(X_j) = \left\{
    \begin{array}{rl}
      1-p_j&\text{ if }X_j=0\\
      1&\text{ if }X_j=1,
    \end{array}\right. \quad
  F_j^\leftarrow(u) = \left\{
    \begin{array}{rl}
      0&\text{ if }0<u\le 1-p_j\\
      1&\text{ if }1-p_j<u\le 1,
    \end{array}\right.
\end{equation*}
for all $0<u<1$. Remember that $X_j = F_j^\leftarrow(\Phi(Z_j))$,
$j=1,2$, where $Z_1$ and $Z_2$ are standard normal random variables
with correlation $\rho$. Remember also that $Z_1=Z_2$ almost surely
(that is, with probability one) if and only if $\rho=1$, and
$Z_1=-Z_2$ almost surely if and only if $\rho=-1$. Let
$X_1 \sim \mathcal{B}(p_1)$.

\emph{Case~(ii).} For the first claim of the proposition, note that  
$(X_1,\mathbf{1}_{\{X_2>F_2^{-1}(1-p_1)\}})$ is comonotonic if and
only if $\Pr(X_1=0, X_2>F_2^{-1}(1-p_1)) + \Pr(X_1=1, X_2\le
F_2^{-1}(1-p_1)) = 0$. This implies
\begin{align*}
  0 &= \Pr(X_1=0, X_2>F_2^{-1}(1-p_1))\\
    &= \Pr(F_1^\leftarrow(\Phi(Z_1))=0, \Phi(Z_2)>1-p_1)\\
    &= \Pr(Z_1\le \Phi^{-1}(1-p_1), Z_2>\Phi^{-1}(1-p_1)),
\end{align*}
which is false unless $\rho=1$. Conversely, if $\rho=1$ then $Z_1=Z_2$
almost surely and
\begin{align*}
  &\Pr(X_1=0, X_2\le F_2(1-p_1)) + \Pr(X_1=1, X_2>F_2^{-1}(1-p_1))\\
  &= \Pr(F_1^\leftarrow(\Phi(Z_1))=0, \Phi(Z_1)\le 1-p_1) + \Pr(F_1^\leftarrow(\Phi(Z_1))=1,
    \Phi(Z_1)>1-p_1)\\
  &= \Pr(\Phi(Z_1)\le 1-p_1) + \Pr(\Phi(Z_1)>1-p_1)\\
  &= 1.
\end{align*}
For the second claim of the proposition, note that
$(X_1,\mathbf{1}_{\{X_2> F_2^{-1}(p_1)\}})$ is countermonotonic if and
only if
$\Pr(X_1=0, X_2\le F_2^{-1}(p_1)) + \Pr(X_1=1, X_2> F_2^{-1}(p_1))
= 0$. This implies $\Pr(\Phi(Z_1)\le 1-p_1, \Phi(Z_2)\le p_1) = 0$, which
is false unless $\rho=-1$. Conversely, if $\rho=-1$ then
\begin{align*}
  &\Pr(X_1=0, X_2> F_2^{-1}(p_1)) + \Pr(X_1=1, X_2\le F_2^{-1}(p_1))\\
  &= \Pr(\Phi(Z_1)\le 1-p_1, \Phi(-Z_1)> p_1) + \Pr(\Phi(Z_1)>1-p_1,
    \Phi(-Z_1)\le p_1)\\
  &= \Pr(\Phi(Z_1)\le 1-p_1) + \Pr(\Phi(Z_1)>1-p_1)\\
  &= 1.
\end{align*}
This proves case~(ii).

\emph{Case~(iii).} For the first claim of the proposition, note that
$X_1\le X_2$ almost surely if and only if $\Pr(X_1=1, X_2=0) = 0$. But
\begin{align*}
  \Pr(X_1=1, X_2=0)
  &= \Pr(F_1^\leftarrow(\Phi(Z_1))=1, F_2^\leftarrow(\Phi(Z_2))=0)\\
  &= \Pr(1-p_1<\Phi(Z_1), \Phi(Z_2)\le 1-p_2),
\end{align*}
which is null if and only if $\rho=1$ (because $p_1\le p_2$). For the
second claim of the proposition, note that $X_1+X_2>0$ almost surely
if and only if
\begin{equation*}
  0 = \Pr(X_1=0, X_2=0) =
  \Pr(\Phi(Z_1)\le 1-p_1, \Phi(Z_2)\le 1-p_2).
\end{equation*}
Since $\Phi^{-1}(1-p_1)\le -\Phi^{-1}(1-p_2)$, the latter probability
is null if and only if $\rho=-1$.

 \section{Correlation coefficient computation}
 \label{appendix:pearson}
 Let $X \sim \mathcal{N}(0,3)$ and $Y=\mathbb{1}_{\{X\geq t\}}$ for a
 given threshold $t$. Let us show first that $(X,Y)$ belongs to
 model~(\ref{eqn:model}). Let $F$ and $G$ denote the CDFs of $X$ and
 $Y$, respectively. We know that $F(x) = \Phi(x/\sqrt{3})$ and
 \begin{equation*}
   G(y) = \left\{\begin{array}{rl}
                   0 & \text{ if }y<0\\
                   \Phi(t/\sqrt{3}) & \text{ if }0\le y<1\\
                   1 & \text{ otherwise}.
                 \end{array}\right.
             \end{equation*}
 It is easy to see that
 \begin{equation*}
   G^{\leftarrow}(u) =
   \left\{
     \begin{array}{rl}
       0 & \text{ if }0<u\le\Phi(t/\sqrt{3})\\
       1 & \text{ otherwise. }
     \end{array}\right.
 \end{equation*}
 for all $u \in (0,1]$.            
 It suffices to exhibit a standard Gaussian random vector $(Z_1,Z_2)$
 with correlation $\rho$
 such that $X = F^{\leftarrow}(\Phi(Z_1))$ and $Y =
 G^{\leftarrow}(\Phi(Z_2))$. But this is easily checked for $\rho=1$.

It is known that the Pearson correlation coefficient between $X$ and $Y$ is given by:
 $$\rho^P(X,Y)=\dfrac{\mathbb{E}[(X-\mathbb{E}(X))(Y-\mathbb{E}(Y))]}{\sigma(X)\sigma(Y)}$$
 where $\mathbb{E}(X)$ (resp. $\mathbb{E}(Y)$) denotes the expectation of $X$ (resp. $Y$) and $\sigma(X)$ (resp. $\sigma(Y)$) denotes the standard deviation of $X$ (resp. $Y$). We know that $\mathbb{E}(X)=0$ and $\sigma(X)=\sqrt{3}$. Moreover, we have
 \begin{eqnarray*}
   \mathbb{E}(Y)&=\mathbb{E}(\mathbb{1}_{\{X\geq t\}})\\
                &=\mathbb{P}(X\geq t)\\
                &=1-\Phi(\frac{t}{\sqrt{3}})
 \end{eqnarray*}
 and $\sigma(Y)=\sqrt{\Phi(\frac{t}{\sqrt{3}})(1-\Phi(\frac{t}{\sqrt{3}}))}$ because we can recognize that $Y \sim \mathcal{B}(1-\Phi(\frac{t}{\sqrt{3}}))$. Hence, we get:
 \begin{eqnarray*}
   \rho^P(X,Y)&=&\dfrac{\mathbb{E}[(X-\mathbb{E}(X))(Y-\mathbb{E}(Y))]}{\sigma(X)\sigma(Y)}\\
              &=&\dfrac{\mathbb{E}[X(Y-1+\Phi(\frac{t}{\sqrt{3}}))]}{\sqrt{3\Phi(\frac{t}{\sqrt{3}})(1-\Phi(\frac{t}{\sqrt{3}}))}}\\
              &=&\dfrac{\mathbb{E}(XY)-\mathbb{E}(X)+\Phi(\frac{t}{\sqrt{3}})\mathbb{E}(X)}{\sqrt{3\Phi(\frac{t}{\sqrt{3}})(1-\Phi(\frac{t}{\sqrt{3}}))}}\\
   &=&\dfrac{\mathbb{E}(XY)}{\sqrt{3\Phi(\frac{t}{\sqrt{3}})(1-\Phi(\frac{t}{\sqrt{3}}))}}.
 \end{eqnarray*}
 Let us compute $\mathbb{E}(XY)$.
 \begin{eqnarray*}
   \mathbb{E}(XY)&=&\mathbb{E}(X\mathbb{1}_{\{X\geq t\}})\\
                &=&\int_{-\infty}^{\infty}x\mathbb{1}_{\{x\geq t\}}\frac{1}{\sqrt{3\times 2 \pi}}\exp(\frac{-x^2}{2\times 3})dx\\
                 &=&\int_{t}^{\infty}x\frac{1}{\sqrt{6\pi}}\exp(\frac{-x^2}{6})dx\\
                 &=&[\dfrac{-3}{\sqrt{6\pi}}\exp(\frac{-x^2}{6})]^{+\infty}_t\\
   &=&\dfrac{3}{\sqrt{6\pi}}\exp(\frac{-t^2}{6}).
 \end{eqnarray*}
 So we end up with
 $$\rho^P(X,Y)=\dfrac{\exp(\frac{-t^2}{6})}{\sqrt{2\pi\Phi(\frac{t}{\sqrt{3}})(1-\Phi(\frac{t}{\sqrt{3}}))}}.$$
 Similarly, Spearman's rho is given by
 $$\rho^s(X,Y)=\dfrac{\mathbb{E}[(F(X)-\mathbb{E}(F(X)))(G(Y)-\mathbb{E}(G(Y)))]}{\sigma(F(X))\sigma(G(Y))}.$$ We have
 \begin{eqnarray*}
   \mathbb{E}(G(Y))&=&\Phi(\frac{t}{\sqrt{3}})\mathbb{P}(Y=0)+\mathbb{P}(Y=1)\\
                &=&\Phi(\frac{t}{\sqrt{3}})^2+1-\Phi(\frac{t}{\sqrt{3}})
 \end{eqnarray*}
 and by the same reasoning, $\mathbb{E}(G(Y)^2)=\Phi(\frac{t}{\sqrt{3}})^3+1-\Phi(\frac{t}{\sqrt{3}})$, which leads to
 \begin{eqnarray*}
   \mathbb{\sigma}(G(Y))&=&\sqrt{\mathrm{Var}(G(Y))}\\
                &=&\sqrt{\mathbb{E}(G(Y)^2)-\mathbb{E}(G(Y))^2}\\
                        &=&\sqrt{\Phi(\frac{t}{\sqrt{3}})^3+1-\Phi(\frac{t}{\sqrt{3}})-[\Phi(\frac{t}{\sqrt{3}})^2+1-\Phi(\frac{t}{\sqrt{3}})]^2}\\
   &=&\sqrt{-\Phi(\frac{t}{\sqrt{3}})^4+3\Phi(\frac{t}{\sqrt{3}})^3-3\Phi(\frac{t}{\sqrt{3}})^2+\Phi(\frac{t}{\sqrt{3}})}
 \end{eqnarray*}
 Moreover, we know that $F(X) \sim \mathcal{U}[0,1]$ so $\mathbb{E}(F(X))=\dfrac{1}{2}$ and $\mathbb{\sigma}(F(X))=\sqrt{\dfrac{1}{12}}$.

 So, we get:
 \begin{eqnarray*}
   \rho^S(X,Y)&=&\dfrac{\mathbb{E}[(F(X)-\mathbb{E}(F(X)))(G(Y)-\mathbb{E}(G(Y)))]}{\sigma(F(X))\sigma(G(Y))}\\
              &=&\dfrac{\mathbb{E}[(F(X)G(Y)]-\mathbb{E}(F)\mathbb{E}(G)}{\sqrt{\frac{1}{12}(-\Phi(\frac{t}{\sqrt{3}})^4+3\Phi(\frac{t}{\sqrt{3}})^3-3\Phi(\frac{t}{\sqrt{3}})^2+\Phi(\frac{t}{\sqrt{3}}))}}\\
   &=&\dfrac{\mathbb{E}[(F(X)G(Y)]-\frac{1}{2}(\Phi(\frac{t}{\sqrt{3}})^2+1-\Phi(\frac{t}{\sqrt{3}}))}{\sqrt{\frac{1}{12}(-\Phi(\frac{t}{\sqrt{3}})^4+3\Phi(\frac{t}{\sqrt{3}})^3-3\Phi(\frac{t}{\sqrt{3}})^2+\Phi(\frac{t}{\sqrt{3}}))}}
 \end{eqnarray*}
 Let us compute $\mathbb{E}(F(X)G(Y))$.
 \begin{eqnarray*}
   \mathbb{E}(F(X)G(Y))&=&\mathbb{E}(F(X)G(\mathbb{1}_{\{X\geq t\}}))\\
                &=&\int_{-\infty}^{\infty}\Phi(\frac{x}{\sqrt{3}})G(\mathbb{1}_{\{x\geq t\}})\frac{1}{\sqrt{3\times 2 \pi}}\exp(\frac{-x^2}{2\times 3})dx\\
                       &=&\int_{-\infty}^{t}\Phi(\frac{x}{\sqrt{3}})\Phi(\frac{t}{\sqrt{3}})\frac{1}{\sqrt{6\pi}}\exp(\frac{-x^2}{6})dx+\int_{t}^{\infty}\Phi(\frac{x}{\sqrt{3}})\frac{1}{\sqrt{6\pi}}\exp(\frac{-x^2}{6})dx\\
                       &=&[\dfrac{\Phi^2(\frac{x}{\sqrt{3}})\Phi(\frac{t}{\sqrt{3}})}{2}]^t_{-\infty} + [\dfrac{\Phi^2(\frac{x}{\sqrt{3}})}{2}]^{+\infty}_t\\
   &=& \dfrac{1+\Phi^3(\frac{t}{\sqrt{3}})-\Phi^2(\frac{t}{\sqrt{3}})}{2}
\end{eqnarray*}
 So we end up with
 $$\rho^S(X,Y)=\dfrac{\Phi^3(\frac{t}{\sqrt{3}})-2\Phi^2(\frac{t}{\sqrt{3}})+\Phi(\frac{t}{\sqrt{3}})}{\sqrt{\frac{1}{3}(-\Phi(\frac{t}{\sqrt{3}})^4+3\Phi(\frac{t}{\sqrt{3}})^3-3\Phi(\frac{t}{\sqrt{3}})^2)}}.$$

%%%%%%%%%%%%%%%%%%%%%%%%%%%%%%%%%%%%%%%%%%%%%%%%%%%%%%%%%%%%%%%%%%%%%%%
\bibliographystyle{abbrvnat}
\bibliography{biblio.bib}

\end{document}
